# Supplementary material for: Narrowing your FOV with SOLiD: Spatially Organized and Lightweight Global Descriptor for FOV-constrained LiDAR Place Recognition
Source: arXiv:2408.07330 source file (2024-10-02)
Supplement: Supplementary file 1 [file author_response.tex]

% Copyright Javier Sánchez-Monedero.
% Please report bugs and suggestions to (jsanchezm at uco.es)
%
% This document is released under a Creative Commons Licence
% CC-BY-SA (http://creativecommons.org/licenses/by-sa/3.0/)
%
% BASIC INSTRUCTIONS:
% 1. Load and set up proper language packages
% 2. Complete the paper data commands
% 3. Use commands \rcomment and \newtext as shown in the example

\documentclass[a4paper,twoside,10pt]{reviewresponse}

% 1. Load and set up proper language packages
%\usepackage[utf8x]{inputenc}
%\usepackage[latin9]{inputenc}
\usepackage[T1]{fontenc}
\usepackage[english]{babel}

%\usepackage{url}
\usepackage{subfigure}
\usepackage{enumitem}
\usepackage{graphicx}
\usepackage{natbib}
\usepackage{amsmath,amssymb,psfrag,color}
\usepackage{soul} % allows text markup symbols like strikethrough (\textst)
\usepackage{multirow}
\usepackage{booktabs}

\usepackage{kotex}

% for highlighting
\usepackage{soul,color}
\newcommand{\bl}[1]{{\textcolor{blue}{#1}}}
\definecolor{gl}{HTML}{008000}
\newcommand{\gl}[1]{{\textcolor{gl}{#1}}}

\DeclareMathOperator*{\argmin}{argmin}
\DeclareMathOperator*{\median}{median}

% table
\usepackage[symbol]{footmisc}
\usepackage{caption}

\usepackage{../Packages/sparo_math}
\usepackage{../Packages/sparo_misc}
\usepackage{../Packages/sparo_acronyms}
\usepackage{../Packages/sparo_SIunits}

\renewcommand{\thefigure}{\Alph{figure}}

%\usepackage{hyperref}
% custom markup commands for response to reviewers
\newcommand{\tflag}[1]{\marginpar{\hspace*{-1mm}\color{red}\scriptsize\bf{\fbox{#1}}}}
\newcommand{\tfflag}[1]{{\color{red}\scriptsize\bf{\fbox{#1}}}}

\newcommand{\cc}[1]{{\color{red}{\bf Co-Authors:} #1}}

% \thanks{${}^{1}$ H. Kim, ${}^{1}$ J. Choi, and ${}^{1*}$ Y. Cho are with the Dept. Electr. and Comput. Eng., Inha University, South Korea \texttt{(e-mail: [hg.kim, jiwon2]@inha.edu, yg.cho@inha.ac.kr)} \newline ${}^{2}$ T. Sim is with the Dept. Electr. Eng., Inha University, South Korea \texttt{(e-mail: xogn2359@gmail.com)} \newline ${}^{3}$ G. Kim is with Vision Group of NAVER LABS, Seongnam, Gyeonggi-do, 13561, Republic of Korea \texttt{(e-mail: giseop.kim@naverlabs.com)}}

% 2. Complete the paper data
\newcommand{\myAuthors}{{Hogyun Kim$^{\displaystyle 1}$, Jiwon Choi$^{\displaystyle 1}$, Taehu Sim$^{\displaystyle 2}$, Giseop Kim$^{\displaystyle 3}$, and Younggun Cho$^{\displaystyle 1\dagger}$}}
\newcommand{\myAuthorsShort}{Hogyun Kim, Jiwon Choi, Taehu Sim, Giseop Kim, and Younggun Cho}
\newcommand{\myEmail}{hg.kim@inha.edu, jiwon2@inha.edu, xogn2359@gmail.com, giseop.kim@naverlabs.com, yg.cho@inha.ac.kr}
\newcommand{\myTitle}{Appendix}
\newcommand{\myShortTitle}{IEEE Robotics and Automation Letters}
% \newcommand{\myShortTitle}{Response to reviewers}
\newcommand{\myJournal}{Narrowing your FOV with SOLiD: Spatially Organized and Lightweight Global Descriptor for FOV-constrained LiDAR Place Recognition}
\newcommand{\myDept}{{$^{\displaystyle 1}$Inha University, Electrical and Computer Engineering}\\ 
                     {$^{\displaystyle 2}$Inha University, Electrical Engineering}\\
                     {$^{\displaystyle 3}$Vision Group of NAVER LABS, Seongnam, Gyeonggi-do, 13561, Republic of Korea}}
%%%%%%%%%%%%%%%%%%%%%%%%%%%%%%%%%%%%%%%%%%%%%%%%%%%%%%%%%%%%%%%%%%%%%%%%%%

% Single day experience based long-term LiDAR localization using Urban Visibility Metric

%\usepackage[linktoc=all]{hyperref}
\usepackage[linktoc=all,bookmarks,bookmarksopen=true,bookmarksnumbered=true]{hyperref}

\hypersetup{
pdfauthor = {\myAuthorsShort},
pdftitle = {\myTitle},
pdfsubject = {\myJournal\xspace},
colorlinks = true,
linkcolor=black!70!green,          % color of internal links
citecolor=black!70!green,        % color of links to bibliography
filecolor=magenta,      % color of file links
urlcolor=black!70!green           % color of external links
}

\begin{document}

\thispagestyle{plain}

\begin{center}
 {\LARGE\myTitle} \vspace{0.5cm} \\
 {\large\myJournal} \vspace{0.5cm} \\
 \today \vspace{0.5cm} \\
 \myAuthors \\
 \url{\myEmail} \vspace{1cm} \\
 \myDept  \vspace{0.5cm}
\end{center}

\section{Full View (360$\circ$) Results}

We evaluate Recall@1, AUC score, F1 max score, and time as shown in \tabref{table:eval_pr}.
Ring++ outperforms in all performance evaluation metrics, followed by LoGG3D and ours.
However, Ring++ lags in terms of speed, making it unsuitable for real-time SLAM or multi-robot systems.
On the other hand, our method can achieve both speed and performance.
Especially in terms of AUC score per unit weight, as represented in Fig. 1 of this paper, our method also overwhelmingly outperforms the results of the full 360-degree view.

\begin{table*}[h]
\caption{Peformance Evaluation for Full View LiDAR Place Recognition}
\renewcommand{\arraystretch}{1.2}
\centering\resizebox{\textwidth}{!}{
\begin{tabular}{cccccccccccccc}
\toprule \hline
\multicolumn{14}{c}{Sequence}                                                                                                                                                                                                                                                                                                                                                                                               \\ \hline
\multicolumn{1}{c|}{\multirow{2}{*}{Method}}   & \multicolumn{1}{c|}{\multirow{2}{*}{Size [bytes]$\big\downarrow$}} & \multicolumn{4}{c|}{00 (4541 frames)}  & \multicolumn{4}{c|}{02 (4661 frames)} & \multicolumn{4}{c}{05 (2761 frames)}\\ \cline{3-14} 
\multicolumn{1}{c|}{}             & \multicolumn{1}{c|}{}  & Recall@1 $\uparrow$ & \multicolumn{1}{c}{AUC $\uparrow$} & \multicolumn{1}{c}{F1 max $\uparrow$} & \multicolumn{1}{c|}{Time [Hz] $\uparrow$}                                                        & \multicolumn{1}{c}{Recall@1 $\uparrow$}      & \multicolumn{1}{c}{AUC $\uparrow$} & \multicolumn{1}{c}{F1 max $\uparrow$} & \multicolumn{1}{c|}{Time [Hz] $\uparrow$} 
                                  & \multicolumn{1}{c}{Recall@1 $\uparrow$}      & \multicolumn{1}{c}{AUC $\uparrow$} & \multicolumn{1}{c}{F1 max $\uparrow$} & Time [Hz] $\uparrow$ \\ \hline
\multicolumn{1}{c|}{Hist. (C)}        & \multicolumn{1}{c|}{\textbf{928}}        & \multicolumn{1}{c}{0.817}               &0.983                    &0.808                       & \multicolumn{1}{c|}{0.58}          
                                                                                 & 0.433                                   &0.963                    &0.427                       & \multicolumn{1}{c|}{0.58}     
                                                                                 & 0.544                                   &\textbf{0.976}           &0.598                       & 0.58     \\
\multicolumn{1}{c|}{Logg3D (G)}       & \multicolumn{1}{c|}{2176}                & \multicolumn{1}{c}{\textbf{0.918}}      &0.982                    &0.879                       & \multicolumn{1}{c|}{15.8}
                                                                                 & \textbf{0.881}                          &\textbf{0.978}           &\textbf{0.801}              & \multicolumn{1}{c|}{15.8}
                                                                                 & \textbf{0.912}                          &0.965                    &\textbf{0.836}              &  16.5    \\
\multicolumn{1}{c|}{M2DP (C)}         & \multicolumn{1}{c|}{1664}                & \multicolumn{1}{c}{0.829}               &0.987                    &0.839                       & \multicolumn{1}{c|}{3.31}
                                                                                 & 0.677                                   &0.968                    &0.706                       & \multicolumn{1}{c|}{3.31}
                                                                                 & 0.625                                   &0.965                    &0.673                       & 3.34     \\
\multicolumn{1}{c|}{SC (C)}           & \multicolumn{1}{c|}{10016}               & \multicolumn{1}{c}{0.893}               &0.979                    &0.876                       & \multicolumn{1}{c|}{3.04}
                                                                                 & 0.794                                   &0.946                    &0.778                       & \multicolumn{1}{c|}{3.04}
                                                                                 & 0.742                                   &0.968                    &0.785                       & 3.09   \\
\multicolumn{1}{c|}{OT (G)}           & \multicolumn{1}{c|}{1152}                & \multicolumn{1}{c}{0.904}               &0.981                    &0.863                       & \multicolumn{1}{c|}{\textbf{\bl{44.8}}}
                                                                                 & 0.782                                   &0.962                    &0.759                       & \multicolumn{1}{c|}{\textbf{\bl{44.6}}}
                                                                                 & 0.857                                   &0.960                    &0.750                       & \textbf{\bl{47.6}}     \\

\multicolumn{1}{c|}{CVT-NET (G)}      & \multicolumn{1}{c|}{3200}                & \multicolumn{1}{c}{0.845}               &0.988                    &0.875                       & \multicolumn{1}{c|}{8.08}
                                                                                 & 0.811                                   &0.954                    &0.807                       & \multicolumn{1}{c|}{8.07}
                                                                                 & 0.702                                   &0.975                    &0.753                       & 8.17     \\

\multicolumn{1}{c|}{Ring++ (G)}       & \multicolumn{1}{c|}{345728}              & \multicolumn{1}{c}{\textbf{\bl{0.954}}} &\textbf{\bl{0.997}}      &\textbf{\bl{0.937}}         & \multicolumn{1}{c|}{0.44}
                                                                                 & \textbf{\bl{0.959}}                     &\textbf{\bl{0.988}}      &\textbf{\bl{0.877}}         & \multicolumn{1}{c|}{0.43}
                                                                                 & \textbf{\bl{0.962}}                     &\textbf{\bl{0.988}}      &\textbf{\bl{0.938}}         & 0.72    \\
\multicolumn{1}{c|}{Ours (C)}         & \multicolumn{1}{c|}{\textbf{\bl{448}}}   & \multicolumn{1}{c}{0.863}               &\textbf{0.996}           &\textbf{0.900}              & \multicolumn{1}{c|}{\textbf{20.8}}
                                                                                 & 0.765                                   &0.965                    &0.799                       & \multicolumn{1}{c|}{\textbf{20.8}}
                                                                                 & 0.776                                   &0.961                    &0.767                       & \textbf{22.1}    \\ \hline \bottomrule
\multicolumn{14}{r}{$^{\mathrm{*}}$ \textbf{\bl{first rank}} is blue and \textbf{second rank} is bold.} \\

\end{tabular}}
\vspace{-0.5cm}
\label{table:eval_pr}
\end{table*}

\section{Downsampling}
We evaluated the performance through an ablation study, as shown in the \tabref{table:voxel}. 

\begin{table*}[h]
\caption{Performance Evaluation according to voxel size of downsampling in KITTI 00}
\renewcommand{\arraystretch}{1.2}
\centering\resizebox{\textwidth}{!}{
\begin{tabular}{cccccccccccccc}
\toprule \hline
\multicolumn{11}{c}{FOV}                                                                                                                                                                                                                                                                                                                                                                                               \\ \hline
\multicolumn{1}{c|}{\multirow{2}{*}{Method}}   & \multicolumn{1}{c|}{\multirow{2}{*}{Voxel Size}} & \multicolumn{3}{c|}{60$^\circ$}  & \multicolumn{3}{c|}{120$^\circ$} & \multicolumn{3}{c}{180$^\circ$}\\ \cline{3-11} 
\multicolumn{1}{c|}{}  & \multicolumn{1}{c|}{}  & Recall@1 $\uparrow$                     & \multicolumn{1}{c}{AUC $\uparrow$} & \multicolumn{1}{c|}{F1 max $\uparrow$}                                                              & \multicolumn{1}{c}{Recall@1 $\uparrow$} & \multicolumn{1}{c}{AUC $\uparrow$} & \multicolumn{1}{c|}{F1 max $\uparrow$} 
                                                & \multicolumn{1}{c}{Recall@1 $\uparrow$} & \multicolumn{1}{c}{AUC $\uparrow$} & \multicolumn{1}{c}{F1 max $\uparrow$}  \\ \hline
                                  
\multicolumn{1}{c|}{Ours (Modified)}   & \multicolumn{1}{c|}{0.1m}  & \multicolumn{1}{c}{0.765}      &0.971                               &\multicolumn{1}{c|}{0.762}
                                                                    & 0.791                          &0.983                               &\multicolumn{1}{c|}{0.807}  
                                                                    & 0.793                          &0.982                               &0.799                       \\

\multicolumn{1}{c|}{Ours}              & \multicolumn{1}{c|}{0.5m}  & \multicolumn{1}{c}{\textbf{\bl{0.800}}}      &\textbf{\bl{0.986}}   &\multicolumn{1}{c|}{\textbf{\bl{0.830}}}
                                                                    & 0.822                          &\textbf{\bl{0.994}}                 &\multicolumn{1}{c|}{\textbf{\bl{0.867}}}  
                                                                    & \textbf{\bl{0.840}}            &\textbf{\bl{0.994}}                 &\textbf{\bl{0.868}}           \\

\multicolumn{1}{c|}{Ours (Modified)}   & \multicolumn{1}{c|}{1.0m}  & \multicolumn{1}{c}{0.798}      &0.978                               &\multicolumn{1}{c|}{0.778}
                                                                    & \textbf{\bl{0.830}}            &0.987                               &\multicolumn{1}{c|}{0.822}  
                                                                    & \textbf{\bl{0.840}}            &0.987                               &0.826                       \\ \hline \bottomrule 
\multicolumn{11}{r}{$^{\mathrm{*}}$ \textbf{\bl{first rank}} is blue.} \\

\end{tabular}}
\label{table:voxel}
\end{table*}

\noindent We found that 0.5m and 1.0m perform the best, in that order. 
Note that the proposed approach performs similarly under different voxel resolutions (0.5m and 1m). 
We also tested our method with a minimal (0.1m) voxel size.
These cases yielded weaker performance than the best cases, but the metrics did not drop significantly.

\section{RAC}
We can create a Radial-Azimuthal bin (i.e. Bird-eye view (BEV)) with elevational projection to utilize \textit{RAC (Radial-Azimuthal Counter)}.
If we use \textit{RAC} for a place recognition problem, we create an \textit{IAV (Implicit Azimuth Counter)} or \textit{IRV (Implicit Range Counter)}.
Similar to \textit{R-SOLiD} with rotation invariance for loop detection, the matrix product between \textit{RAC} and \textit{IAV} generates \textit{R-RAC}.
The experiments were conducted with the Aeva LiDAR, which has the smallest vertical FOV, to ensure minimal impact of vertical information.
\tabref{table:ablation_rac} shows that vertical information is meaningful for representing narrow FOV.
    
\begin{table*}[h]
\caption{Peformance Evaluation in HeLiPR with Aeva LiDAR}
\renewcommand{\arraystretch}{1.2}
\centering\resizebox{\textwidth}{!}{
\begin{tabular}{cccccccccccccc}
\toprule \hline
\multicolumn{11}{c}{Sequence}                                                                                                                                                                                                                                                                                                                                                                                               \\ \hline
\multicolumn{1}{c|}{\multirow{2}{*}{Method}}   & \multicolumn{1}{c|}{\multirow{2}{*}{Size [bytes]$\big\downarrow$}} & \multicolumn{3}{c|}{Town01-Town02}  & \multicolumn{3}{c|}{RoundAbout01-RoundAbout02} & \multicolumn{3}{c}{KAIST04-KAIST05}\\ \cline{3-11} 
\multicolumn{1}{c|}{}  & \multicolumn{1}{c|}{}  & Recall@1 $\uparrow$                     & \multicolumn{1}{c}{AUC $\uparrow$} & \multicolumn{1}{c|}{F1 max $\uparrow$}                                                              & \multicolumn{1}{c}{Recall@1 $\uparrow$} & \multicolumn{1}{c}{AUC $\uparrow$} & \multicolumn{1}{c|}{F1 max $\uparrow$} 
                                                & \multicolumn{1}{c}{Recall@1 $\uparrow$} & \multicolumn{1}{c}{AUC $\uparrow$} & \multicolumn{1}{c}{F1 max $\uparrow$}  \\ \hline
                                  
\multicolumn{1}{c|}{R-SOLiD using RAC}  & \multicolumn{1}{c|}{448}   & \multicolumn{1}{c}{0.733}      &0.907                               &\multicolumn{1}{c|}{0.733}
                                                         & 0.697                          &0.830                               &\multicolumn{1}{c|}{0.605}  
                                                         & 0.872                          &0.936                               &0.877                       \\
                                                                                 

\multicolumn{1}{c|}{R-SOLiD using REC}& \multicolumn{1}{c|}{448}   & \multicolumn{1}{c}{\textbf{\bl{{0.781}}}} &\textbf{\bl{0.934}}       &\multicolumn{1}{c|}{\textbf{\bl{0.783}}}
                                                         & \textbf{\bl{0.729}}                       &\textbf{\bl{0.886}}       &\multicolumn{1}{c|}{\textbf{\bl{0.646}}} 
                                                         & \textbf{\bl{0.882}}                       &\textbf{\bl{0.955}}       &\textbf{\bl{0.886}}     \\ \hline \bottomrule 

\multicolumn{11}{r}{$^{\mathrm{*}}$ \textbf{\bl{first rank}} is blue.} \\

\end{tabular}}
% \vspace{-0.5cm}
\label{table:ablation_rac}
\end{table*}
    
\section{3-D matching graph in HeLiPR datasets}
We draw a 3-D graph when the F1 score is maximized and when the precision is 100$\%$.
For methods where precision does not reach 100$\%$, we base the graph on the highest precision achieved.
In the Aeva sequence, the proposed method exhibits the densest matching performance, while in the Avia sequence, RING++ demonstrates the densest matching performance.

%% Matching Graph
%% ===========================================================================================================================================================================
\begin{figure*}[h]
    \centering
    \def\width{0.98\columnwidth}
    \includegraphics[clip, trim= 0 250 0 60, width=\width]{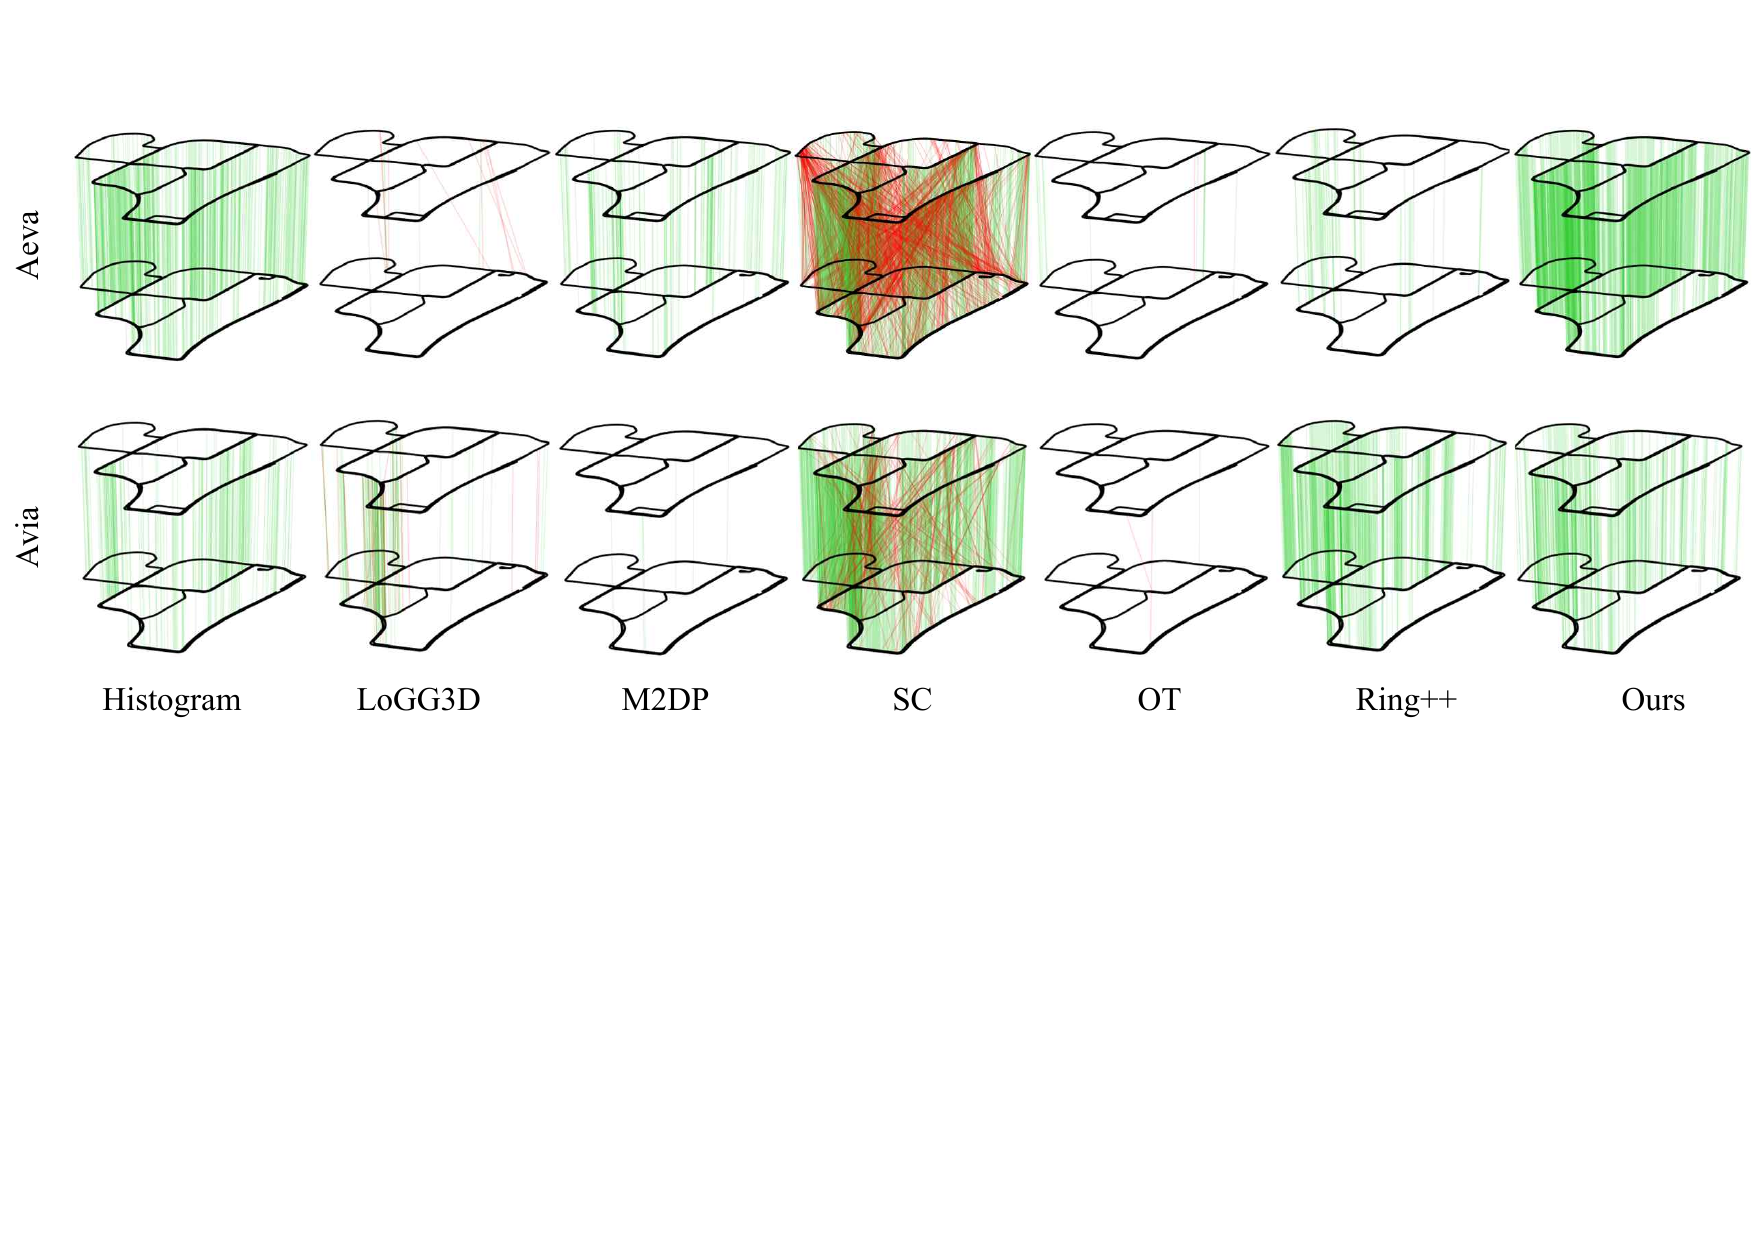}
    \caption{3-D matching pair graph when each descriptor's precision is highest in \textit{HeLiPR} dataset (source: \textit{KAIST04}, target: \textit{KAIST05}). Green represents true matching pairs, and red represents false matching pairs.}
    \vspace{-0.5cm}
    \label{fig:matching_Graph}
\end{figure*}
%% ===========================================================================================================================================================================

\section{Constant IEV}
To check the impact of IEV, we compare the results when using constant IEV as the ablation study.

\begin{table*}[h]
\caption{Peformance Evaluation in KITTI 05 with Constant IEV}
\renewcommand{\arraystretch}{1.2}
\centering\resizebox{\textwidth}{!}{
\begin{tabular}{cccccccccccccc}
\toprule \hline
\multicolumn{11}{c}{FOV}                                                                                                                                                                                                                                                                                                                                                                                               \\ \hline
\multicolumn{1}{c|}{\multirow{2}{*}{Method}}   & \multicolumn{1}{c|}{\multirow{2}{*}{Size [bytes]$\big\downarrow$}} & \multicolumn{3}{c|}{60$^\circ$}  & \multicolumn{3}{c|}{120$^\circ$} & \multicolumn{3}{c}{180$^\circ$}\\ \cline{3-11} 
\multicolumn{1}{c|}{}  & \multicolumn{1}{c|}{}  & Recall@1 $\uparrow$                     & \multicolumn{1}{c}{AUC $\uparrow$} & \multicolumn{1}{c|}{F1 max $\uparrow$}                                                              & \multicolumn{1}{c}{Recall@1 $\uparrow$} & \multicolumn{1}{c}{AUC $\uparrow$} & \multicolumn{1}{c|}{F1 max $\uparrow$} 
                                                & \multicolumn{1}{c}{Recall@1 $\uparrow$} & \multicolumn{1}{c}{AUC $\uparrow$} & \multicolumn{1}{c}{F1 max $\uparrow$}  \\ \hline
                                  
\multicolumn{1}{c|}{Ours-Constant IEV}  & \multicolumn{1}{c|}{448}  & \multicolumn{1}{c}{0.635}      &0.988                               &\multicolumn{1}{c|}{0.731}
                                                                    & 0.652                          &0.987                               &\multicolumn{1}{c|}{0.732}  
                                                                    & 0.657                          &0.965                               &0.693                       \\
                                                                                 

\multicolumn{1}{c|}{Ours}               & \multicolumn{1}{c|}{448}  & \multicolumn{1}{c}{\textbf{\bl{{0.639}}}} &\textbf{\bl{0.992}}       &\multicolumn{1}{c|}{\textbf{\bl{0.732}}}
                                                                    & \textbf{\bl{0.656}}                       &\textbf{\bl{0.989}}       &\multicolumn{1}{c|}{\textbf{\bl{0.737}}} 
                                                                    & \textbf{\bl{0.659}}                       &\textbf{\bl{0.974}}       &\textbf{\bl{0.710}}  \\ \hline \bottomrule 

\multicolumn{11}{r}{$^{\mathrm{*}}$ \textbf{\bl{first rank}} is blue.} \\

\end{tabular}}
\label{table:constant_iev}
\end{table*}

\end{document}
